# Supplementary material for: Alpine Permafrost Modeling: On the influence of topography driven lateral fluxes
Source: arXiv:2110.07217 source file (2021-10-18)
Supplement: Supplementary file 1 [file supplementary_material.tex]

%\section*{Supplementary Material}
%Nothing yet 
